# Supplementary material for: LOGIC-LM++: Multi-Step Refinement for Symbolic Formulations
Source: arXiv:2407.02514 source file (2024-08-06)
Supplement: Supplementary file 1 [file appendix.tex]

\section{Appendix}
\label{sec:appendix}

\begin{figure}[h]
\centering
\begin{promptbox}
\justify
""" \\
\{
    "name": "Problem Formulator", \\
    "description": "Task Quality gauges the degree to which a model adheres to and executes the specific directives given in the prompt. This metric zeroes in exclusively on the fidelity of the model's response to the prompt's instructions. An ideal response not only recognizes the overt commands of the prompt but also respects its nuance and subtleties. The scoring rubric is described below, with a few possible reasons (which might not be exhaustive) for a given score.", \\
    "scoring": \{ \\
        "0": \{ \\
            "(a)": "The model disregards the instructions entirely.", \\
            "(b)": "The output is entirely irrelevant to the prompt.", \\
            "(c)": "There is a clear disconnect between the user's request and the model's response." \\
        \}, \\
        "1": \{ \\
            "(a)": "The model grasps and addresses the main theme or element of the instruction but may miss out on finer details or nuances.", \\
            "(b)": "There is partial alignment with the prompt, indicating some elements of relevance, but not a complete match.", \\
            "(c)": "The response might include extraneous details not asked for, or it might omit some requested specifics." \\
        \}, \\
        "2": \{ \\
            "(a)": "The model demonstrates a precise understanding and adherence to the prompt's instructions.", \\
            "(b)": "The output holistically satisfies all aspects of the given directive without any deviation.", \\
            "(c)": "There's a clear and direct correlation between the user's instruction and the model's response, with no aspect of the instruction left unaddressed."
        \}
    \}
\} \\
"""
\end{promptbox}
\caption{Task Quality metric rubric}
\label{fig:task-quality-prompt}
\end{figure}
